# Supplementary material for: Human Activity Recognition in an Open World
Source: arXiv:2212.12141 source file (2025-01-15)
Supplement: Supplementary file 1 [file class_balance.tex]

\section{Visualize Class Balance}

\begin{figure*}[t]
    \centering
    \includegraphics[width=1.0\linewidth]{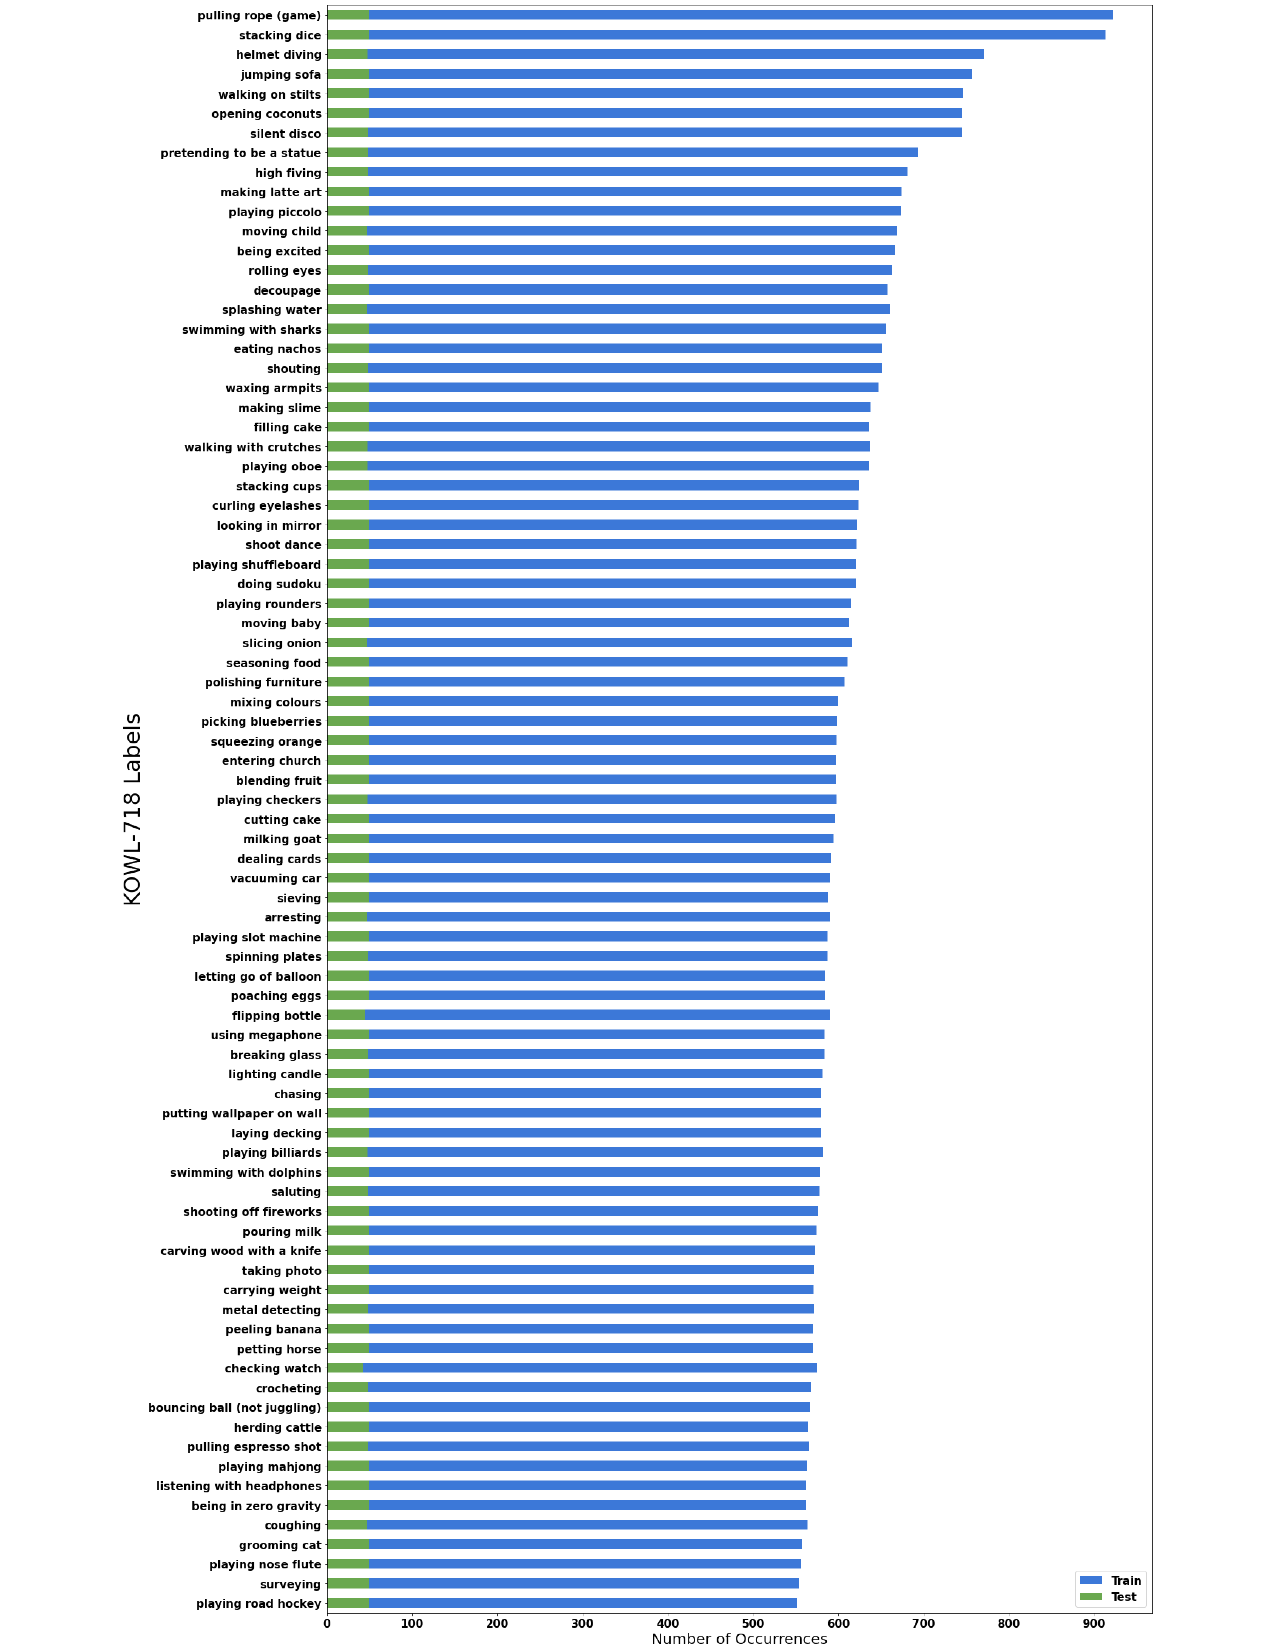}
    \iffalse
    \caption{
        KOWL-718 class balance.
    }
    \fi
\label{sm:sec:ava}
\end{figure*}
