# Supplementary material for: Human Activity Recognition in an Open World
Source: arXiv:2212.12141 source file (2025-01-15)
Supplement: Supplementary file 2 [file supp_mat.tex]

\input{writing/3.1_novelty_set_relations}
\input{writing/appendix/experiments}
